# Supplementary material for: Adaptive estimating function inference for non-stationary determinantal point processes
Source: arXiv:1806.06231 ancillary file (2019-11-15)
Supplement: Supplementary file 1 [file eeGeneral-supplementary.pdf]

# Supplementary material for "Adaptive estimating function inference for non-stationary determinantal point processes"

FRÉDÉRIC LAVANCIER[1,*] ARNAUD POINAS[2,**] RASMUS WAAGEPETERSEN[3,†]

[1] *Laboratoire de Mathématiques Jean Leray – BP 92208 – 2, Rue de la Houssinière – F-44322 Nantes Cedex 03 – France. Inria, Centre Rennes Bretagne Atlantique, France.*
E-mail: [*] frederic.lavancier@univ-nantes.fr

[2] *IRMAR – Campus de Beaulieu - Bat. 22/23 – 263 avenue du Général Leclerc – 35042 Rennes – France*
E-mail: [**] arnaud.poinas@univ-rennes1.fr

[3] *Department of Mathematical Sciences – Aalborg University - Fredrik Bajersvej 7G – DK-9220 Aalborg – Denmark*
E-mail: [†] rw@math.aau.dk

## 1. Supplementary tables for Section 4.1 of the main manuscript

For the simulation study carried out in Section 4.1 of the main manuscript, considering estimation for a DPP model with a Bessel-type kernel, we report in Figure S1 the boxplots representing the distribution of the estimators and in Table S1 the percentages of times each estimation method has converged in our simulation study. These percentages are similar for all estimation methods. Table S2 displays the root mean square errors of the estimators considered in Section 4.1 where, for comparison, we also include results for the adaptive estimator using $\varepsilon = 0.05$. Conclusions based on these tables are given in the main paper.

## 2. Two-step versus simultaneous

Referring to Section 4.2, Figure S2 shows how irregular the contrast function $e(\psi)$ for the simultaneous approach can be in comparison with the contrast function $e_2(\psi)$ for the two-step approach. The underlying point pattern is displayed on the left. This is

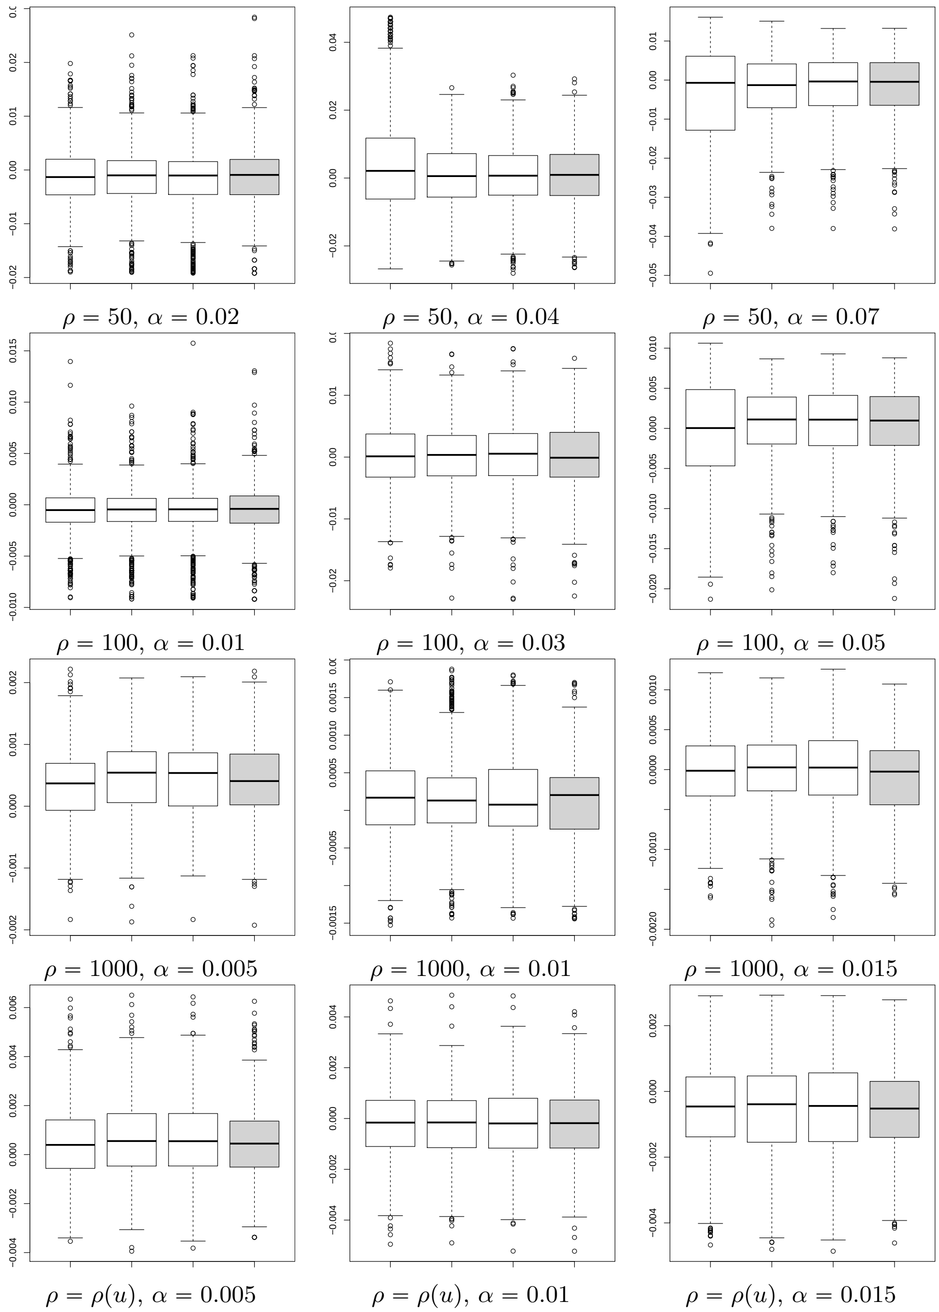


**Figure S1**. Distribution of $\hat{\alpha} - \alpha$ for a Bessel-type DPP on $[0, 1]^2$ for different values of $\rho$ and $\alpha$. In each subfigure, the 3 first estimators on the left use the test function (3) of the main manuscript with $R = 0.05$, $R = 0.1$ and $R = 0.25$ respectively, while the last estimator is the adaptive version based on (4).

| $\rho$ | $\alpha$ | $R = 0.05$ | $R = 0.1$ | $R = 0.25$ | Adaptive |
|---|---|---|---|---|---|
| 50 | 0.02 | 0.75 | 0.72 | 0.72 | 0.72 |
| | 0.04 | 0.97 | 0.85 | 0.80 | 0.85 |
| | 0.07 | 0.92 | 1.00 | 0.99 | 0.98 |
| 100 | 0.01 | 0.66 | 0.69 | 0.72 | 0.64 |
| | 0.03 | 0.99 | 0.96 | 0.89 | 0.93 |
| | 0.05 | 1.00 | 1.00 | 1.00 | 1.00 |
| 1000 | 0.005 | 1.00 | 0.95 | 0.95 | 0.95 |
| | 0.01 | 1.00 | 1.00 | 1.00 | 1.00 |
| | 0.015 | 1.00 | 1.00 | 1.00 | 1.00 |
| Inhom | 0.005 | 0.93 | 0.92 | 0.95 | 0.93 |
| | 0.01 | 0.98 | 0.98 | 0.98 | 0.96 |
| | 0.015 | 1.00 | 1.00 | 1.00 | 1.00 |

**Table S1.** Percentage of times the estimation methods have converged for the models and estimators considered in Section 4.1 of the main manuscript.

| $\rho$ | $\alpha$ | $R = 0.05$ | $R = 0.1$ | $R = 0.25$ | $\varepsilon = 0.01$ | $\varepsilon = 0.05$ |
|---|---|---|---|---|---|---|
| 50 | 0.02 | 5.49 | 5.45 | 5.95 | 5.53 | 7.13 |
| | 0.04 | 14.92 | 8.81 | 8.79 | 8.87 | 8.71 |
| | 0.07 | 13.08 | 8.10 | 8.07 | 8.04 | 8.82 |
| 100 | 0.01 | 2.30 | 2.27 | 2.45 | 2.49 | 2.77 |
| | 0.03 | 5.05 | 4.99 | 5.16 | 5.10 | 5.27 |
| | 0.05 | 5.75 | 4.40 | 4.47 | 4.50 | 5.10 |
| 1000 | 0.005 | 0.68 | 0.87 | 0.83 | 0.73 | 0.73 |
| | 0.01 | 0.57 | 0.59 | 0.61 | 0.56 | 0.59 |
| | 0.015 | 0.47 | 0.46 | 0.52 | 0.47 | 0.51 |
| Inhom | 0.005 | 1.58 | 1.65 | 1.66 | 1.61 | 1.57 |
| | 0.01 | 1.34 | 1.36 | 1.36 | 1.32 | 1.37 |
| | 0.015 | 1.43 | 1.47 | 1.48 | 1.40 | 1.46 |

**Table S2.** RMSE ($\times 10^3$) for the same simulations as in Table 1 of the main manuscript, with the addition of the adaptive estimator using $\varepsilon = 0.05$. These quantities are computed from 1000 simulations where all five estimation methods have converged (explaining the differences with Table 1 of the main manuscript).

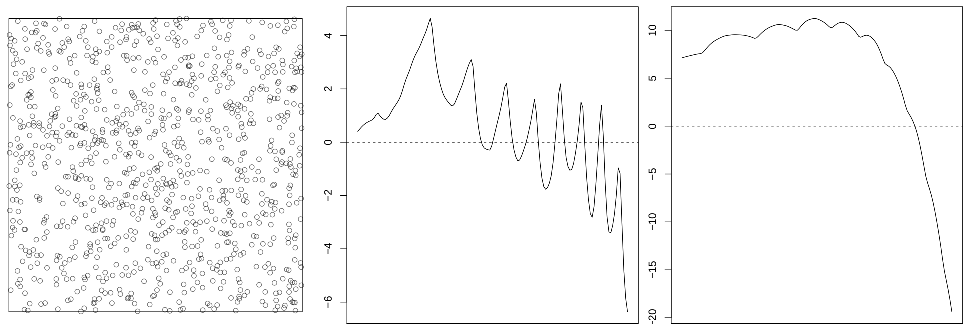


**Figure S2**. Realization of a DPP (left) and plots of the contrast function $e(\psi)$ (see (9) in the main manuscript) of the simultaneous procedure (middle) and of the contrast function $e_2(\psi)$ (see (8)) of the two-step procedure (right) obtained for the data in the left plot.

a realisation on the unit square of a homogeneous DPP with a Gaussian kernel, with intensity $\rho = 1000$ and range $\alpha = 0.01$.

Figure S3 reports the distributions of estimates of $\rho$ over 1000 realisations on the unit square of a DPP with a Bessel-type kernel with $\rho = 1000$ and $\alpha = 0.01$. The two first estimators come from the simultaneous approach, see equation (10) of the main manuscript where $\hat{\psi} = \hat{\alpha}$ in this setting. For the first one, the numerical solution of $e(\alpha) = 0$ to get $\hat{\alpha}$ was initialized at the true value 0.01 of $\alpha$. For the second one, $\hat{\alpha}$ was fixed to the true value, i.e. $\hat{\alpha} = 0.01$. The last estimator on the right of Figure S3 is simply $\hat{\rho} = N(X \cap W)/|W|$, corresponding to the first step of the two-step procedure. The respective root mean square errors are 33.6, 31.4 and 26. See the main manuscript for further discussion.

# 3. Some simulations for the Thomas model

The adaptive estimating function is also useful for clustered point processes. Here we consider a Thomas model on $[0,1]^2$, with parent intensity $\kappa = 100$, offspring intensity $\mu = 10$ and various values of the dispersal kernel standard deviation $\sigma$. The same three estimation methods as in Section 4.1 of the main manuscript have been evaluated, where for the adaptive version both $\varepsilon = 0.01$ and $\varepsilon = 0.05$ have been considered. A point pattern sample and the distribution of the estimators of $\kappa$ and $\sigma$ based on 1000 replications are shown in Figure 3 for $\sigma = 0.02$, $\sigma = 0.035$ and $\sigma = 0.05$ respectively. Estimators of the library `spatstat` [1] of `R` [2] with default settings have also been added. These are: minimum contrast estimation based on the $K$-function, Guan's composite likelihood, and Palm likelihood, see also Section 2.3 in the main manuscript. Table S3 summarises the estimated root mean square errors for each estimation method.

Also for the Thomas process, the adaptive method, both with $\varepsilon = 0.01$ and $\varepsilon = 0.05$, performs well compared with the three fixed $R$ estimators. In fact for $\sigma = 0.05$, the

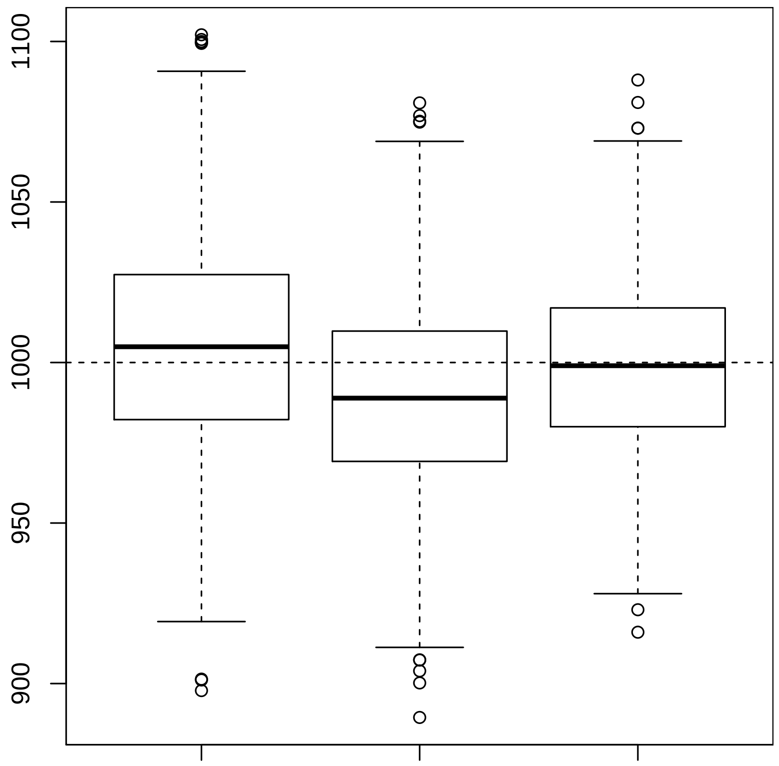


**Figure S3**. Distribution of estimates of $\rho$ obtained from 1000 realisations of the Bessel-type DPP on $W = [0, 1]^2$ with $\rho = 1000$ and $\alpha = 0.01$. Left: the simultaneous estimator as given in equation (10) with initial value for the numerical solution given by the true value 0.01 of $\alpha$. Middle: as left but using the true value of $\alpha$ instead of $\hat{\alpha}$. Right: $\hat{\rho} = N(X \cap W)/|W|$ corresponding to the first step of a two-step procedure.

| $\sigma$ | | $R = 0.05$ | $R = 0.1$ | $R = 0.25$ | $\varepsilon = 0.01$ | $\varepsilon = 0.05$ | $K$ | clik | Palm |
|---|---|---|---|---|---|---|---|---|---|
| 0.02 | $\hat{\kappa}$ | 17 | 21 | 21 | 21 | 20 | 23 | 28 | 21 |
| | | (0.40) | (0.48) | (0.47) | (0.48) | (0.47) | (0.54) | (0.70) | (0.49) |
| | $\hat{\sigma}$ | 1.04 | 1.84 | 1.94 | 1.79 | 1.51 | 2.60 | 1.54 | 1.92 |
| | | (0.02) | (0.06) | (0.08) | (0.07) | (0.04) | (0.09) | (0.03) | (0.09) |
| 0.035 | $\hat{\kappa}$ | 35 | 31 | 40 | 38 | 35 | 33 | 121 | 35 |
| | | (0.79) | (0.75) | (0.95) | (0.89) | (0.85) | (0.81) | (4.20) | (0.90) |
| | $\hat{\sigma}$ | 4.80 | 5.54 | 7.92 | 6.24 | 4.59 | 5.76 | 8.04 | 5.50 |
| | | (0.09) | (0.14) | (0.32) | (0.21) | (0.10) | (0.14) | (0.07) | (0.12) |
| 0.05 | $\hat{\kappa}$ | 54 | 49 | 53 | 47 | 53 | 35 | 554 | 39 |
| | | (1.24) | (0.92) | (2.05) | (1.74) | (1.89) | (1.55) | (13.64) | (1.02) |
| | $\hat{\sigma}$ | 18.30 | 36.47 | 12.17 | 11.22 | 8.94 | 8.12 | 23.69 | 19.47 |
| | | (1.28) | (1.47) | (0.41) | (0.53) | (0.61) | (0.25) | (0.13) | (0.74) |

**Table S3.** For the Thomas model, estimated root mean square errors of various estimators of $\kappa$ and $\sigma$ ($\times 10^3$). The 3 first estimators use the test function (3) of the main manuscript with $R = 0.05$, $R = 0.1$ and $R = 0.25$ respectively; the fourth and fifth estimators are the adaptive version based on (4) where $\varepsilon = 0.01$ and $\varepsilon = 0.05$; the three last estimators are from the library `spatstat`: based on $K$, on Guan's composite likelihood (clik) and on Palm likelihood - all with default settings. The standard errors of the MSE estimations are given in parenthesis.

adaptive versions are better than any of the fixed $R$ estimators. The adaptive method also has good stable performance compared with the three `spatstat` methods. In particular, the adaptive method performs much better than Guan's composite likelihood with default settings.

# References

[1] Baddeley, A. J., Rubak, E. and Turner, R. (2015). *Spatial Point Patterns: Methodology and Applications with R. Interdisciplinary Statistics*. Chapman & Hall/CRC, Boca Raton, Florida.

[2] R Core Team (2017). R: A Language and Environment for Statistical Computing R Foundation for Statistical Computing, Vienna, Austria.

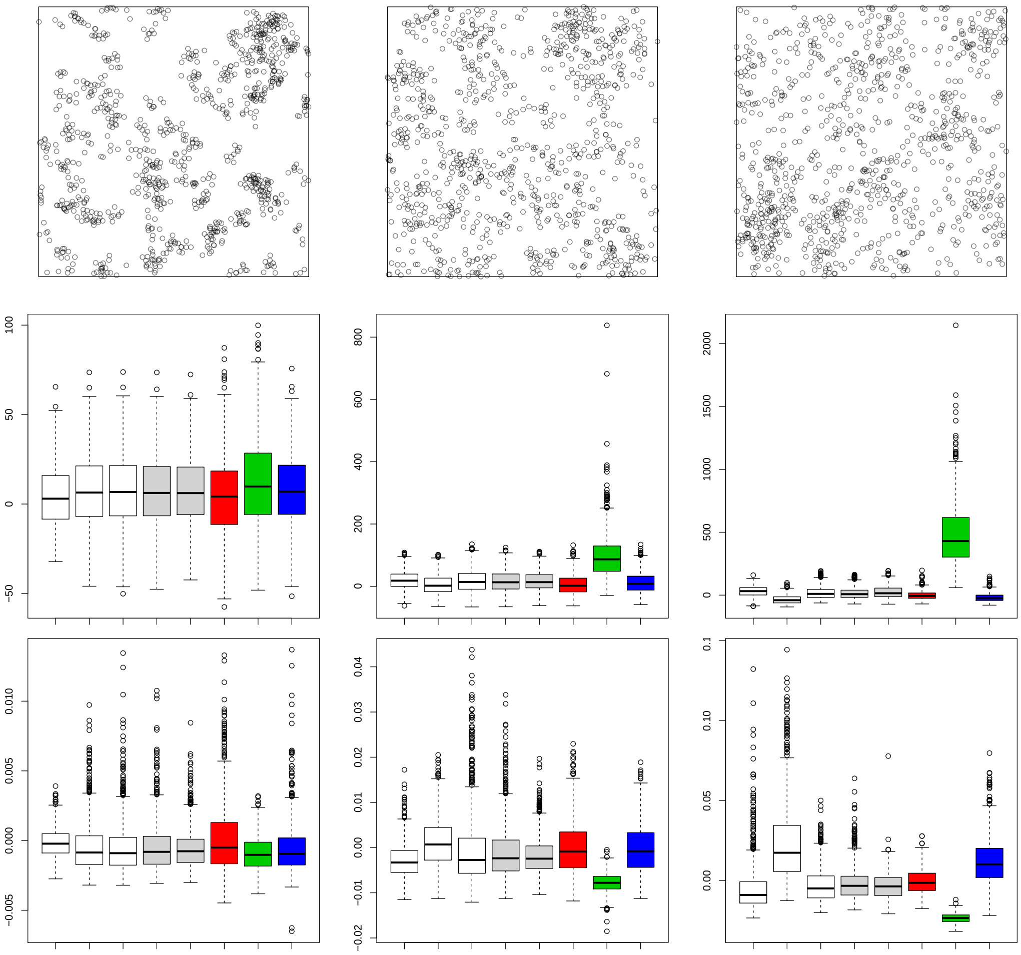

**Figure S4**. First row: Examples of point patterns simulated from a Thomas model on $[0,1]^2$ for $\kappa = 100$, $\mu = 10$ and from left to right $\sigma = 0.02, 0.035, 0.05$. Second row: Distribution of estimates of $\kappa$ based on 1000 replications. In each plot, the 3 first boxplots are for estimates obtained with the test function (3) of the main manuscript with $R = 0.05$, $R = 0.1$ and $R = 0.25$ respectively; the fourth and fifth boxplots (in grey) are for the adaptive version based on (4) where $\varepsilon = 0.01$ (left) and $\varepsilon = 0.05$ (right); the three last boxplots are for methods from `spatstat`: based on $K$ (red), on Guan's composite likelihood (green) and on Palm likelihood (blue) - all with default settings. Third row: Distribution of estimates of $\sigma$ based on 1000 replications, using the same estimation methods.
